# Supplementary material for: PLM: Efficient Peripheral Language Models Hardware-Co-Designed for Ubiquitous Computing
Source: arXiv:2503.12167 source file (2025-03-19)
Supplement: Supplementary file 2 [file hardware_deployment.tex]

\section{Hardware Deployment}
